# Supplementary material for: Situation Monitor: Diversity-Driven Zero-Shot Out-of-Distribution Detection using Budding Ensemble Architecture for Object Detection
Source: arXiv:2406.03188 source file (2024-06-05)
Supplement: Supplementary file 1 [file supplementary.tex]

\section{Supplementary}

\subsection{Extension of Situation Monitor on Unseen Novel Objects}
In this section, we utilize the KITTI dataset to explore the Situation Monitor's (SM) capability in detecting novel, unseen objects within the same dataset. Specifically, to establish an optimal setup and ideal configuration, the training dataset intentionally omits any images containing instances of unseen objects, with their inclusion reserved exclusively for the validation and evaluation phases of both the model and the Situation Monitor. 
Consequently, we transition from $\mathcal{O^\textit{near}}$ and $\mathcal{O^\textit{far}}$ datasets problem statement to $\mathcal{O^\textit{near}}$ and $\mathcal{O^\textit{far}}$ objects. 
Our experimental approach encompasses two distinct sets. The first set involves the removal of van and truck classes during the training phase, while images containing these classes are introduced exclusively during the evaluation phase. In this set, van and truck classes can be considered as $\mathcal{O^\textit{near}}$ objects, given the continued presence of the car class in the training data, which shares similarities with vans and trucks.
Conversely, the second set of experiments focuses on removing person sitting, pedestrian, and cyclist classes during training. In this set, these two objects are categorized as $\mathcal{O^\textit{far}}$ objects, as there is no resemblance between these objects and any others present in the training data. This meticulous experimental design allows for a nuanced assessment of the Situation Monitor's performance across various object classes and distances.

Furthermore, the final OOD value $\mathcal{U}_{SM}$ will now be monitored at the object level, departing from the earlier image-level approach as detailed in Section \ref{situation_monitor} and Eq. \eqref{eq:OOD_final}. In this object-level monitoring, there is no longer a need to compute the mean of object variances or centre the variances to maintain OOD values at the object level. This shift is attributed to the inclusion of raw variances, which encapsulate localization errors crucial for capturing novel objects. Despite this adjustment, the confidence score $C$ of the detection remains instrumental in centring the variances. The refined $\mathcal{U}_{SM}$ monitoring values, as shown in Eq. \eqref{eq:OOD_final_object} enhances the Situation Monitor's efficacy in identifying and characterizing novel objects within the given context.
For evaluating the situation monitor on unseen novel objects, we categorise the detections that overlap with the unseen objects using the ground truth as a novel OOD object. The detections are the in-distribution objects; otherwise, they don't belong to these unseen novel object categories but are true positives.
To assess the Situation Monitor's performance on unseen novel objects during training, we categorize detections that overlap with the ground truth of these unseen objects as novel Out-of-Distribution (OOD) objects. In contrast, in-distribution objects are detections that neither belong to the category of these unseen novel objects nor are considered false positives, indicating accurate identification.

\begin{equation}
\label{eq:OOD_final_object}
\begin{aligned}
   xy_{var} = \sqrt{\sum_{i \in (x, y)}{(b^{\alpha}_{i} - b^{\beta}_{i}})^2}, \\
   wh_{var} = \sum_{i \in (w, h)}{(b^{\alpha}_{i} - b^{\beta}_{i}})^2, \\
   \mathcal{U}_{SM} = \frac{\sqrt{xy_{var}}*wh_{_var}}{\sqrt{C}}
\end{aligned}
\end{equation}`

\begin{figure}[h]
\centering     %%% not \center
\subfigure[Vans and trucks classes as $\mathcal{O^\textit{near}}$ objects]{\label{fig:ex_SM_ped}\includegraphics[width=0.45\columnwidth]{icml2024/images/suppl/Exten_SM_Van.png}}
\subfigure[Pedestrians, person sitting and Cyclists classes as $\mathcal{O^\textit{far}}$ objects]{\label{fig:ex_SM_van}\includegraphics[width=0.45\columnwidth]{icml2024/images/suppl/Exten_SM_Ped.png}}
\caption{Images showing the instances of unseen novel objects considered to study the extension of the situation monitor}
\label{fig:images_extension_SM}
\end{figure}

\subsubsection{Van and trucks classes as $\mathcal{O^\textit{near}}$ objects}

\begin{figure}[h]
\centering     %%% not \center
\subfigure[]{\label{fig:ex_SM_ped}\includegraphics[width=0.45\columnwidth]{icml2024/images/suppl/suppl_van_truck_all_metrics.png}}
\subfigure[]{\label{fig:ex_SM_van}\includegraphics[width=0.45\columnwidth]{icml2024/images/suppl/suppl_van_truck_auroc_hist.png}}
\caption{Metrics evaluating the Situation Monitor's detection of $\mathcal{O^\textit{near}}$ objects (Vans and trucks classes)}
\label{fig:supp_near_ood}
\end{figure}

The findings in Figure \ref{fig:supp_near_ood} indicate that the Situation Monitor (SM) faces challenges in identifying the Van and Truck classes as novel objects. This observation aligns seamlessly with the conceptual framework of SM refraining from categorizing the Near-OOD ($\mathcal{O^\textit{near}}$) as Out-of-Distribution (OOD). 
This difficulty distinguishing Van and Truck classes as novel objects stems from the inherent resemblance between their features and those of the familiar Car class.

\subsubsection{Pedestrians, person sitting and Cyclists classes as $\mathcal{O^\textit{near}}$ objects}

In many training processes, the common practice is to initiate training using pre-trained weights. These weights are often derived from well-established datasets such as CoCo or ImageNet, containing classes that may align with $\mathcal{O}^\textit{far}$. Consequently, this initialization can impact the model's ability to detect unseen objects during real-time inference, even if these objects were not part of the training dataset.
In such scenarios, the significance of an OOD detector becomes pronounced. This detector plays a crucial role in classifying novel or unseen objects, especially in safety-critical situations where previously not encountered instances require accurate identification for effective decision-making and response. The capability to distinguish and appropriately handle unforeseen objects enhances the overall robustness and reliability of the model in real-world applications.

Conversely, maintaining an ideal configuration for the setup involves training without the utilization of pre-trained weights. Instead, the model is trained from scratch, initializing the weights randomly. However, this approach does not guarantee that the model will refrain from detecting unseen objects, as illustrated in Figure \ref{fig:ped_det_NPT}, which are not part of the ground truth. Ground truth typically refers to the annotated or labelled objects the model has been trained on. If an object is present in an image but is not part of the training data, the DNN may still attempt to identify and classify it based on learned features.

\begin{figure}[h]
\centering     %%% not \center
\subfigure[Inference on sample images using model trained with no pre-trained weights]{\label{fig:ex_SM_ped}\includegraphics[width=\columnwidth]{icml2024/images/suppl/ped_det_NPT.png}}
\subfigure[Inference on sample images using model trained with pre-trained weights]{\label{fig:ex_SM_van}\includegraphics[width=\columnwidth]{icml2024/images/suppl/ped_det.png}}
\caption{Visualizing the impact of pre-trained weights on previously unseen and novel objects that are not part of the training dataset.}
\label{fig:ped_det_NPT}
\end{figure}

In the majority of model training procedures, pre-trained weights are commonly used. Hence, we will assess the SM's capability to detect $\mathcal{O^\textit{far}}$ objects on a model trained with these pre-trained weights.
\begin{figure}[h]
\centering     %%% not \center
\subfigure[]{\label{fig:ex_SM_ped}\includegraphics[width=0.45\columnwidth]{icml2024/images/suppl/suppl_ped_all_metrics.png}}
\subfigure[]{\label{fig:ex_SM_van}\includegraphics[width=0.45\columnwidth]{icml2024/images/suppl/suppl_ped_auroc_hist.png}}
\caption{Metrics evaluating the Situation Monitor's detection of $\mathcal{O^\textit{far}}$ objects (Pedestrians, person sitting and Cyclists classes)}
\label{fig:supp_far_ood}
\end{figure}

The outcomes presented in Figure \ref{fig:supp_far_ood} indicate that the performance of the Situation Monitor is not at a particularly high level in detecting $\mathcal{O^\textit{far}}$ objects, as shown in Table \ref{tab:benchmark_results}. However, despite the observed limitations, these results are encouraging, suggesting that there is potential for enhancement, and one avenue for refinement lies in the application of the Diversity-based Budding Ensemble architecture. Implementing this architecture could further elevate the SM's ability to discern and effectively handle instances of FAR-OOD ($\mathcal{O^\textit{far}}$) objects.

Anomalies are apparent in the evaluated CoCo ($\mathcal{O^\textit{far}}$) datasets, displaying characteristics closely resembling either in-distribution datasets or near-OOD $\mathcal{O^\textit{near}}$ datasets. Notably, images related to cars exhibit a closer resemblance to datasets like KITTI, BDD100K, or Cityscapes. This leads to the overlap of $\mathcal{U}_{SM}$ values in Fig. \ref{fig:AUROC_hist_a}. This observation is clearly depicted in Fig. \ref{fig:visual_ood_similar}.

\subsection{More GradCAM examples of DBEA-DINO-DETR}
\begin{figure}[h]
\centering     %%% not \center
\subfigure[]{\label{fig:gradCAM_suppl_1}\includegraphics[width=0.45\columnwidth]{icml2024/images/suppl/Grad_cam_suppl_1.png}}
\subfigure[]{\label{fig:gradCAM_suppl_2}\includegraphics[width=0.45\columnwidth]{icml2024/images/suppl/Grad_cam_suppl_2.png}}
\subfigure[]{\label{fig:gradCAM_suppl_2}\includegraphics[width=0.6\columnwidth]{images/gradCAM_main.png}}
\caption{Visualization of GradCAM on sample images: The top image shows the original detections of DBEA-DINO-DETR. The middle image is the GradCAM image of Vanilla-DINO-DETR.
while the bottom image corresponds to DBEA-DINO-DETR. The color-map on the GradCAM image indicates positive relevance as white and negative relevance as black}
\label{fig:gradCAM_suppl}
\end{figure}

GradCAM visualizations  \cite{selvaraju2017grad}, depicted in Fig. \ref{fig:gradCAM_suppl}, offer valuable insights into the attention and focus areas of the DBEA-based DINO-DETR model. These visualizations illustrate that the model emphasizes specific regions within the image, providing a detailed view of the areas considered crucial for its decision-making process. This heightened focus contributes to the model's improved detection performance and enhances the correlation of its confidence scores. Anomalies in the assessed CoCo ($\mathcal{O^\textit{far}}$) datasets show features resembling either in-distribution datasets or nearby out-of-distribution ($\mathcal{O^\textit{near}}$) datasets, particularly in images related to cars and roads. Thus resulting in overlapping $\mathcal{U}_{SM}$ values in Fig. \ref{fig:AUROC_hist_a}.
